# Supplementary material for: Absence of backscattering in Fermi-arc-mediated conductivity of topological Dirac semimetal Cd$_{3}$As$_{2}$
Source: arXiv:2312.03108 ancillary file (2023-12-05)
Supplement: Supplementary file 1 [file Supplemental_Material.pdf]

# Supplementary Material: Absence of backscattering in Fermi–arc–mediated conductivity of topological Dirac semimetal Cd<sub>3</sub>As<sub>2</sub>

Vsevolod Ivanov<sup>1,2,3</sup>, Lotte Borkowski<sup>4</sup>, Xiangang Wan<sup>5</sup>, and Sergey Y. Savrasov<sup>4</sup>

<sup>1</sup>Virginia Tech National Security Institute, Blacksburg, Virginia 24060, USA

<sup>2</sup>Department of Physics, Virginia Tech, Blacksburg, Virginia 24061, USA

<sup>3</sup>Virginia Tech Center for Quantum Information Science and Engineering, Blacksburg, Virginia 24061, USA

<sup>4</sup>Department of Physics, University of California, Davis, CA 95616, USA

<sup>5</sup>National Laboratory of Solid State Microstructures, School of Physics and Collaborative Innovation Center of Advanced Microstructures, Nanjing University, Nanjing, China

## Supplementary Note 1: Refined Two–Orbital Tight–Binding Model for Cd<sub>3</sub>As<sub>2</sub>

For a general 2x2 Hamiltonian

$$H_{ab}(\mathbf{k}) = \begin{bmatrix} h_{1\mathbf{k}} & v_{\mathbf{k}} \\ v_{\mathbf{k}}^* & h_{2\mathbf{k}} \end{bmatrix},$$

the eigenvalues are given by

$$\epsilon_{1,2}(\mathbf{k}) = \frac{h_{1\mathbf{k}} + h_{2\mathbf{k}}}{2} \mp \frac{1}{2} \sqrt{(h_{1\mathbf{k}} - h_{2\mathbf{k}})^2 + 4|v_{\mathbf{k}}|^2}.$$

If we start from the LDA band structure of Cd<sub>3</sub>As<sub>2</sub>, we have two dispersive bands, therefore

$$\epsilon_2(\mathbf{k}) - \epsilon_1(\mathbf{k}) = \sqrt{(h_{1\mathbf{k}} - h_{2\mathbf{k}})^2 + 4|v_{\mathbf{k}}|^2}.$$

To determine tight binding parameters, we use the following lattice translations of the body centered tetragonal lattice (in units of lattice constants  $a, a, c$  along x,y,z axis)

$$\begin{aligned} A &= (1, 0, 0), \\ B &= (0, 1, 0), \\ C &= (1/2, 1/2, 1/2). \end{aligned}$$

Nearest neighbor vectors from the origin are the following:

$$\begin{aligned} 4 &: R_1 = (\pm 1, 0, 0), (0, \pm 1, 0) \\ 8 &: R_2 = (\pm 1/2, \pm 1/2, \pm 1/2) \\ 2 &: R_3 = (0, 0, \pm 1) \\ 4 &: R_4 = (\pm 1, \pm 1, 0) \\ 8 &: R_5 = (0, \pm 1, \pm 1), (\pm 1, 0, \pm 1) \\ 16 &: R_6 = (\pm 1, \pm 1/2, \pm 1/2), (\pm 1/2, \pm 1, \pm 1/2) \\ 8 &: R_7 = (\pm 1, \pm 1, \pm 1). \end{aligned}$$

Denote  $\epsilon_0 = h(0)$ ,  $t_i = h(R_i)$ . Generally, for  $h(k_x, k_y, k_z)$  obeying full lattice symmetry, we expect that

$$\begin{aligned} h(k_x, k_y, k_z) &= \sum_R e^{ik_x R_x} e^{ik_y R_y} e^{ik_z R_z} h(R_x, R_y, R_z) = \\ &\epsilon_0 + t_1(e^{ik_x a} + e^{-ik_x a} + e^{ik_y a} + e^{-ik_y a}) + \\ &t_2(e^{ik_x a/2} e^{ik_y a/2} e^{ik_z a/2} + \dots) + t_3(e^{ik_z a} + e^{-ik_z a}) \\ &+ t_4(e^{ik_x a/2} e^{ik_y a/2} + e^{ik_x a/2} e^{-ik_y a/2} + e^{-ik_x a/2} e^{ik_y a/2} + e^{-ik_x a/2} e^{-ik_y a/2}) + \dots \\ &= \epsilon_0 + 2t_1(\cos k_x a + \cos k_y a) + \\ &8t_2 \cos k_x a/2 \cos k_y a/2 \cos k_z a/2 + \\ &2t_3 \cos k_z a + 4t_4 \cos k_x a/2 \cos k_y a/2 + \dots \end{aligned}$$

According to the  $k \cdot p$  result, we do not anticipate dispersion of  $v_{\mathbf{k}}$  along 001 line because  $v_{\mathbf{k}} = \lambda(k_x + ik_y)$ . As a result,

$$H_{ab}(0, 0, k_z) = \begin{bmatrix} h_{1\mathbf{k}} & 0 \\ 0 & h_{2\mathbf{k}} \end{bmatrix},$$

and

$$\begin{aligned} \epsilon_1(0, 0, k_z) &= h_1(0, 0, k_z), \\ \epsilon_2(0, 0, k_z) &= h_2(0, 0, k_z). \end{aligned}$$

Thus, the dispersion along 001 determines  $h(0, 0, k_z)$

Denoting  $t_i = h(R_i)$  we obtain along 001 direction:

$$\begin{aligned} h(0, 0, k_z) &= \sum_R e^{ik_z R_z} h(R_x, R_y, R_z) = \epsilon_0 + 4t_1 + 8t_2 \cos k_z a/2 + \\ &\quad 2t_3 \cos k_z a + 4t_4 + 8t_5 \cos k_z a + 16t_6 \cos k_z a/2 + 8t_7 \cos k_z a \\ &= \epsilon_0 + 4(t_1 + t_4) + 8(t_2 + 2t_6) \cos k_z a/2 + 2(t_3 + 4t_5 + 4t_7) \cos k_z a + \dots \end{aligned}$$

For the  $\mathbf{k} = (0, 0, 0)2\pi/a$

$$h(0, 0, 0) = \epsilon_0 + 4(t_1 + t_4) + 8(t_2 + 2t_6) + 2(t_3 + 4t_5 + 4t_7).$$

For the  $\mathbf{k} = (0, 0, 1)2\pi/a$

$$h(0, 0, 1) = \epsilon_0 + 4(t_1 + t_4) - 8(t_2 + 2t_6) + 2(t_3 + 4t_5 + 4t_7).$$

For the  $\mathbf{k} = (0, 0, 1/2)2\pi/a$

$$h(0, 0, 1/2) = \epsilon_0 + 4(t_1 + t_4) - 2(t_3 + 4t_5 + 4t_7).$$

For the  $\mathbf{k} = (0, 0, 1/4)2\pi/a$

$$h(0, 0, 1/4) = \epsilon_0 + 4(t_1 + t_4) + 8(t_2 + 2t_6)/\sqrt{2}.$$

For the  $\mathbf{k} = (0, 0, 3/4)2\pi/a$

$$h(0, 0, 3/4) = \epsilon_0 + 4(t_1 + t_4) - 8(t_2 + 2t_6)/\sqrt{2}.$$

We obtain the following connections between hopping integrals:

$$\begin{aligned} \epsilon_0 + t_1 + t_4 &= [h(0, 0, 0) + h(0, 0, 1) + 2h(0, 0, 1/2)]/16, \\ t_2 + 2t_6 &= [h(0, 0, 0) - h(0, 0, 1)]/16, \\ t_3 + 4t_5 + 4t_7 &= [h(0, 0, 0) + h(0, 0, 1) - 2h(0, 0, 1/2)]/8, \\ \epsilon_0 + t_1 + t_4 &= [h(0, 0, 1/4) + h(0, 0, 3/4)]/8, \\ t_2 + 2t_6 &= [h(0, 0, 1/4) - h(0, 0, 3/4)]\sqrt{2}/16, \end{aligned}$$

We now interpret the above described two orbital model as the two LDA energy bands that cross the Fermi level and produce the Dirac point along  $\Gamma - Z$  line of the Brillouin Zone. We can interpret these two orbitals in the spinor basis of  $|\uparrow\rangle$  and  $|\downarrow\rangle$  states. We use the LDA extracted values for the first band

$$\begin{aligned} \epsilon_1(0, 0, 0) &= 0.02eV, \\ \epsilon_1(0, 0, 1) &= -0.41eV, \\ \epsilon_1(0, 0, 1/2) &= -0.09eV, \\ \epsilon_1(0, 0, 1/4) &= -0.01eV, \\ \epsilon_1(0, 0, 3/4) &= -0.24eV, \end{aligned}$$

which produces

$$\begin{aligned} \epsilon_0^{(1)}/4 + t_1^{(1)} + t_4^{(1)} &= -0.0356eV, \\ t_2^{(1)} + 2t_6^{(1)} &= +0.0269eV, \\ t_3^{(1)} + 4t_5^{(1)} + 4t_7^{(1)} &= -0.0262eV. \end{aligned}$$

We need to use  $\epsilon_0^{(1)} > 0$  so that there is gap everywhere in the BZ except the Dirac point. This gives us the set of on-site energies and hopping integrals for the first orbital:

$$\begin{aligned}\epsilon_0^{(1)} &= 0.1eV, \\ t_1^{(1)} &= -0.0606eV, \\ t_2^{(1)} &= 0.0269eV, \\ t_3^{(1)} &= -0.0262eV,\end{aligned}$$

Similarly, we use the LDA extracted values for the second band:

$$\begin{aligned}\epsilon_2(0,0,0) &= -0.02eV, \\ \epsilon_2(0,0,1) &= 0.55eV, \\ \epsilon_2(0,0,1/2) &= 0.35eV, \\ \epsilon_2(0,0,1/4) &= 0.05eV, \\ \epsilon_2(0,0,3/4) &= 0.50eV,\end{aligned}$$

$$\begin{aligned}\epsilon_0^{(2)}/4 + t_1^{(2)} + t_4^{(2)} &= +0.0769eV, \\ t_2^{(2)} + 2t_6^{(2)} &= -0.0356eV, \\ t_3^{(2)} + 4t_5^{(2)} + 4t_7^{(2)} &= -0.0212eV.\end{aligned}$$

We need to use  $\epsilon_0^{(2)} < 0$  for the fit so that there is gap everywhere in the BZ except the Dirac point. This gives the second set of on-site energies and hopping integrals for the second orbital:

$$\begin{aligned}\epsilon_0^{(2)} &= -0.1eV \\ t_1^{(2)} &= 0.1019eV \\ t_2^{(2)} &= -0.0356eV \\ t_3^{(2)} &= -0.0212eV\end{aligned}$$

Finally in  $k \cdot p$  theory, the off-diagonal parameter between first (spin up) and second (spin down) orbitals  $v(\mathbf{k}) = \lambda(k_x + ik_y)$ . The tight-binding representation that leads to this

$$\begin{aligned}v(\mathbf{k}) &= \sum_{\mathbf{R}} e^{i\mathbf{k}\cdot\mathbf{R}} v(\mathbf{R}) = v(100)e^{ik_x} + v(-100)e^{-ik_x} + v(010)e^{ik_y} + v(0-10)e^{-ik_y} + \\ &\quad v(200)e^{ik_x} + v(-200)e^{-ik_x} + v(020)e^{ik_y} + v(0-20)e^{-ik_y} \\ &= \lambda_1(e^{ik_x} - e^{-ik_x})/2i + \lambda_1 i(e^{ik_x} - e^{-ik_x})/2i + \\ &\quad \lambda_{11}(e^{ik_x}e^{ik_y} - e^{ik_x}e^{-ik_y} - e^{-ik_x}e^{ik_y} + e^{-ik_x}e^{-ik_y})/(2i)^2 \\ &\quad \lambda_2(e^{i2k_x} - e^{-i2k_x})/2i + \lambda_2 i(e^{i2k_x} - e^{-i2k_x})/2i \\ &= \lambda_1(\sin k_x + i \sin k_y) + \lambda_2(\sin 2k_x + i \sin 2k_y).\end{aligned}$$

Here we used

$$\begin{aligned}v(+100) &= +\lambda_1/(2i), \\ v(-100) &= -\lambda_1/(2i), \\ v(0+10) &= +\lambda_1 i/(2i), \\ v(0-10) &= -\lambda_1 i/(2i), \\ \\ v(+200) &= +\lambda_2/(2i), \\ v(-200) &= -\lambda_2/(2i), \\ v(0+20) &= +\lambda_2 i/(2i), \\ v(0-20) &= -\lambda_2 i/(2i).\end{aligned}$$

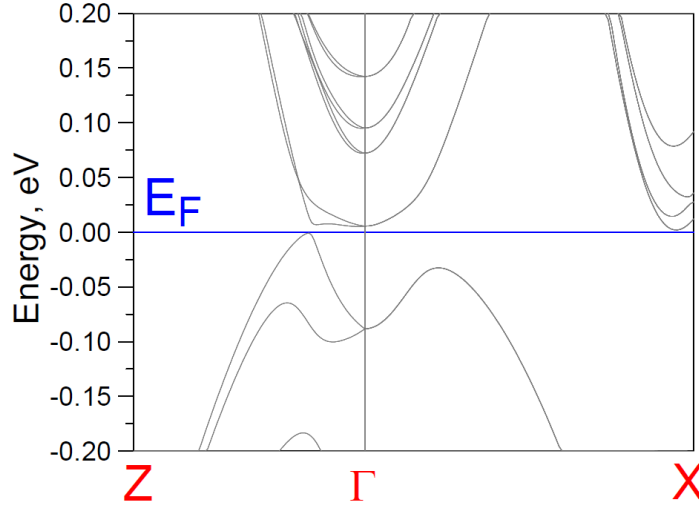

Figure 1: Electronic structure of the distorted  $\text{Cd}_3\text{As}_2$  that shows a gap opening in the vicinity of Dirac points and results in a weak topological insulator phase.

The best fit is obtained with the use of the parameters:

$$\begin{aligned}\lambda_1 &= -0.24\text{eV}, \\ \lambda_2 &= +0.08\text{eV}.\end{aligned}$$

The above parameters are used in our tight-binding simulations of the surface states and the transport properties described in text.

## Supplementary Note 2: Inversion Broken Distorted Structure along (110)

Here we want to describe a symmetry broken phase as caused by a perturbation along 110 crystallographic line. It could be due to the presence of the contact in an experimental setup or strong electric field applied along (110). Such perturbation will break the inversion and leave only 4 symmetry operations of the crystalline group including 180 degrees rotation along (110) as well as reflections within basal and (1-10) planes. Our density functional LDA calculation for such symmetry broken phase involves moving the atoms of Cd and As in the opposite direction along (110) to simulate a compatible distortion. The result is plotted on Fig. 1 where one can see a small gap opening in the vicinity of the Dirac point.

We next analyze this result in terms of a generic  $k \cdot p$  model. For the Dirac semimetal, such model has been described many times in the literature (see, e.g., Phys. Rev. B 88, 125427 (2013)). It consists of two orbitals with  $k$  dispersions  $\pm M(\mathbf{k})$ , where  $M(\mathbf{k}) = M_0 - M_1(k_x^2 + k_y^2) - M_2k_z^2$ , that interact via the matrix element  $A(k_x \pm ik_y)$ . The parameters  $M_0, M_1, M_2$  should be chosen negative to reproduce band inversion. The model naturally respects all symmetry operations of the tetragonal lattice as is the case of the undistorted tetragonal ( $I4_1/acd$ , No.142) structure of  $\text{Cd}_3\text{As}_2$ .

The lowest order  $k \cdot p$  Hamiltonian that illustrates this scenario reads

$$H(\mathbf{k}) = \begin{bmatrix} +M(\mathbf{k}) & A(k_y + ik_x) & 0 & Bk_z \\ A(k_y - ik_x) & -M(\mathbf{k}) & Ck_z & 0 \\ 0 & Ck_z & +M(\mathbf{k}) & -A(k_y - ik_x) \\ Bk_z & 0 & -A(k_y + ik_x) & -M(\mathbf{k}) \end{bmatrix}$$

It describes the transition between Dirac semimetal ( $B = C = 0$ ) and topological insulator ( $B, C \neq 0$ ) phases. If we keep off-diagonal parameters  $B$  and  $C$  different, this describes lifting of the degeneracy along  $\Gamma Z$  (001) line of the BZ as seen in our density functional calculation given in Figure 1.

Next, we convert this  $k \cdot p$  Hamiltonian to the refined four orbital tight-binding model. However, the diagonal  $2 \times 2$  subblocks of this Hamiltonian translate to the two-orbital tight-binding model that we already discussed for the Dirac semimetal phase in the previous section. The off-diagonal terms (the ones with the coefficients  $C$  and  $D$ ) are periodized with the substitution of  $k_z \rightarrow \sin k_z c$ . The numbers  $C$  and  $D$  are small and describe the perturbation that gap the Dirac points and result in the weak topological insulator state of  $\text{Cd}_3\text{As}_2$ . We use its actual values  $C = D = 0.0068$  eV for the plots presented in the main text.
